# Supplementary material for: Exponential Dispersion Models for Overdispersed Zero-Inflated Count Data
Source: arXiv:2003.13854 ancillary file (2020-03-30)
Supplement: Supplementary file 1 [file SupplementEDMforCountData.pdf]

# Supplementary Data Analyses of Exponential Dispersion Models for Overdispersed Zero-Inflated Count Data

Shaul K. Bar-Lev[a] Ad Ridder[b]

[a] *Faculty of Tech. Man., Holon Institute of Technology, Holon, Israel*, shaulb@hit.ac.il
[b] *Department of EOR, VU University, Amsterdam, Netherlands*, ad.ridder@vu.nl

March 31, 2020

**Abstract**

This paper accompanies [1] and [2], in which we developed a framework of discrete distributions based on three classes of exponential dispersion models. In [2] we gave a summary of the extensive data analyses that we executed. This paper contains all our results. For background techniques and notation, for discussion on these data analyses, we refer to [1] and [2].

[1] Bar-Lev, S.K. and A. Ridder (2020a). New exponential dispersion models for count data - properties and applications. Submitted. Available at arXiv.

[2] Bar-Lev, S.K. and A. Ridder (2020b). Exponential dispersion models for overdispersed zero-inflated count data. Submitted. Available at arXiv.

# Part I
# Full Comparison with Reported Fits

Here we present 14 data sets with overdispersion and zero-inflation, which have been considered in literature for developing distributins, and which have been reported for comparison reasons.

## 1 Data Set 1

Insurance claims in Switserland in 1961, see [1].

| value | 0 | 1 | 2 | 3 | 4 | 5 | 6 |
|---|---|---|---|---|---|---|---|
| frequency | 103704 | 14075 | 1766 | 255 | 45 | 6 | 2 |

### 1.1 Literature

[1] Gossiaux, A. and Lemaire, J. (1981). Methodes d'ajustement de distributions de sinistres. *Bulletin of the Association of Swiss Actuaries* 81, 87-95.

[2] Willmot, G. (1987). The Poisson-Inverse Gaussian distribution as an alternative to the negative binomial. *Scandinavian Actuarial Journal* 3-4, 113-127.

[3] Gomez-Deniz, E. and Calderin-Ojeda, E. (2011a). The discrete Lindley distribution: properties and applications. *Journal of Statistical Computation and Simulation* 81, 1405-1416.

### 1.2 Descriptive Statistics

$$\overline{x} = 0.1551,\ s^2 = 0.1793,\ b_1 = 3.154,$$
$$D = 1.558, p_0^{\text{emp}} = 0.8653$$

### 1.3 Fitting Models

[2], [3], [4] ABM($r = 9$), [5] LMS ($r = 3$), and [6] LMNS($r = 1$).

| # of claims | frequency | [2] | [3] | [4] | [5] | [6] |
|---:|---:|---:|---:|---:|---:|---:|
| 0 | 103704 | 103710.03 | 103347.35 | 103719.83 | 103718.88 | 103707.97 |
| 1 | 14075 | 14054.65 | 14628.38 | 14016.51 | 14014.93 | 14060.87 |
| 2 | 1766 | 1784.91 | 1682.27 | 1823.34 | 1827.88 | 1781.15 |
| 3 | 255 | 254.49 | 175.79 | 250.35 | 249.38 | 252.84 |
| 4 | 45 | 40.42 | 17.38 | 36.38 | 35.66 | 40.91 |
| 5 | 6 | 6.94 | 1.65 | 5.55 | 5.31 | 7.40 |
| 6 | 2 | 1.26 | 0.15 | 0.88 | 0.82 | 1.46 |
| $L$ | | -54609.76 | -54659.61 | -54611.59 | -54612.03 | **-54609.75** |
| $\chi^2$ | | 0.7783 | 126.8 | 4.477 | 5.400 | 0.7432 |
| df | | 3 | 4 | 3 | 2 | 3 |
| $p$-value | | 0.8546 | 0.0 | 0.2143 | 0.0672 | **0.8630** |
| RMSE | | 10.89 | 252.8 | 31.75 | 33.34 | **8.182** |

## 2 Data Set 2

Automobile claim data in Great Britain, 1968, see [1].

| value | 0 | 1 | 2 | 3 | 4 | 5 |
|---|---|---|---|---|---|---|
| frequency | 370412 | 46545 | 3935 | 317 | 28 | 3 |

### 2.1 Literature


[1] Gossiaux, A. and Lemaire, J. (1981). Methodes d'ajustement de distributions de sinistres. *Bulletin of the Association of Swiss Actuaries* 81, 87-95.

[2] Willmot, G. (1987). The Poisson-Inverse Gaussian distribution as an alternative to the negative binomial. *Scandinavian Actuarial Journal* 3-4, 113-127.

[3] Gomez-Deniz, E. and Calderin-Ojeda, E. (2011a). The discrete Lindley distribution: properties and applications. *Journal of Statistical Computation and Simulation* 81, 1405-1416.

[4] Gomez-Deniz, E., J.M. Sarabia, and E. Calderin-Ojeda (2011b). A new discrete distribution with actuarial applications. *Insurance: Mathematics and Economics* 48(3), 406-412.


### 2.2 Descriptive Statistics

$$\overline{x} = 0.1317,\ s^2 = 0.1385,\ b_1 = 2.980,$$
$$D = 1.051, p_0^{\text{emp}} = 0.8793$$

### 2.3 Fitting Models

[2], [3], [4], [5] ABM($r = 9$) , [6] LMS($r = 1$), and [7] LMNS($r = 1$).

| # of claims | frequency | [2] | [3] | [4] | [5] | [6] | [7] |
|---|---|---|---|---|---|---|---|
| 0 | 370412 | 370435.00 | 371135.9 | 370412.90 | 370438.64 | 370439.10 | 370434.94 |
| 1 | 46545 | 46476.40 | 45202.2 | 46538.26 | 46460.21 | 46455.72 | 46477.27 |
| 2 | 3935 | 3995.76 | 4464.4 | 3942.39 | 4015.46 | 4022.22 | 3995.05 |
| 3 | 317 | 307.67 | 400.4 | 318.57 | 302.60 | 300.61 | 307.50 |
| 4 | 28 | 23.12 | 33.9 | 25.64 | 21.49 | 20.87 | 23.29 |
| 5 | 3 | 1.74 | 2.7 | 2.06 | 1.49 | 1.39 | 1.80 |
| $L$ | | -171134.4 | -171196.1 | **-171133.3** | -171135.6 | -171136.2 | -171134.4 |
| $\chi^2$ | | 2.744 | 122.4 | 0.3709 | 5.168 | 6.299 | 2.605 |
| df | | 2 | 3 | 2 | 2 | 1 | 2 |
| $p$-value | | 0.2536 | 0.0 | **0.8307** | 0.07548 | 0.01208 | 0.2718 |
| RMSE | | 38.84 | 660.1 | **4.278** | 49.37 | 52.65 | 38.36 |

## 3 Data Set 3

Automobile claim data in Belgium, 1958, see [1].

| value | 0 | 1 | 2 | 3 | 4 | 5 | 6 | 7 |
|---|---|---|---|---|---|---|---|---|
| frequency | 7840 | 1317 | 239 | 42 | 14 | 4 | 4 | 1 |

### 3.1 Literature


[1] Gossiaux, A. and Lemaire, J. (1981). Methodes d'ajustement de distributions de sinistres. *Bulletin of the Association of Swiss Actuaries* 81, 87-95.

[2] Willmot, G. (1987). The Poisson-Inverse Gaussian distribution as an alternative to the negative binomial. *Scandinavian Actuarial Journal* 3-4, 113-127.

[3] Gomez-Deniz, E. and Calderin-Ojeda, E. (2011a). The discrete Lindley distribution: properties and applications. *Journal of Statistical Computation and Simulation* 81, 1405-1416.


### 3.2 Descriptive Statistics

$$\overline{x} = 0.2144,\ s^2 = 0.2889,\ b_1 = 3.481,$$
$$D = 1.348, p_0^{\text{emp}} = 0.8287$$

### 3.3 Fitting Models

[2], [3], [4] ABM($r = 9$) , [5] LMS($r = 4$), and [6] LMNS($r = 1$).

| # of claims | frequency | [2] | [3] | [4] | [5] | [6] |
|---|---|---|---|---|---|---|
| 0 | 7840 | 7844.01 | 7735.57 | 7846.49 | 7854.65 | 7843.38 |
| 1 | 1317 | 1306.12 | 1463.22 | 1295.91 | 1283.34 | 1308.74 |
| 2 | 239 | 238.23 | 225.71 | 247.36 | 249.37 | 236.78 |
| 3 | 42 | 53.27 | 31.67 | 53.84 | 55.37 | 52.24 |
| 4 | 14 | 13.75 | 4.21 | 12.87 | 13.47 | 13.69 |
| 5 | 4 | 3.89 | 0.54 | 3.29 | 3.49 | 4.08 |
| 6 | 4 | 1.17 | 0.07 | 0.89 | 0.95 | 1.34 |
| 7 | 1 | 0.37 | 0.01 | 0.25 | 0.27 | 0.47 |
| $L$ | | -5343.5 | -5377.5 | -5345.0 | -5345.4 | **-5342.9** |
| $\chi^2$ | | 4.536 | 88.66 | 7.750 | 8.211 | 3.375 |
| df | | 3 | 3 | 3 | 2 | 3 |
| $p$-value | | 0.2091 | 0.0 | 0.05148 | 0.01648 | **0.3374** |
| RMSE | | 5.814 | 63.93 | 9.415 | 14.34 | **4.962** |

# 4 Data Set 4

Insurance claims in Zaire in 1974, see [1].

| value | 0 | 1 | 2 | 3 | 4 | 5 |
|---|---|---|---|---|---|---|
| frequency | 3719 | 232 | 38 | 7 | 3 | 1 |

## 4.1 Literature

[1] Gossiaux, A. and Lemaire, J. (1981). Methodes d'ajustement de distributions de sinistres. *Bulletin of the Association of Swiss Actuaries* 81, 87-95.

[2] Willmot, G. (1987). The Poisson-Inverse Gaussian distribution as an alternative to the negative binomial. *Scandinavian Actuarial Journal* 3-4, 113-127.

[3] Gomez-Deniz, E. and Calderin-Ojeda, E. (2011a). The discrete Lindley distribution: properties and applications. *Journal of Statistical Computation and Simulation* 81, 1405-1416.

[4] Gomez-Deniz, E., J.M. Sarabia, and E. Calderin-Ojeda (2011b). A new discrete distribution with actuarial applications. *Insurance: Mathematics and Economics* 48(3), 406-412.

[5] Bhati, D. and H.S. Bakouch (2019). A new infinitely divisible discrete distribution with applications to count data modeling. *Communications in Statistics - Theory and Methods* 48(6), 1401-1416.

## 4.2 Descriptive Statistics

$$\overline{x} = 0.08650,\ s^2 = 0.1225,\ b_1 = 5.316,$$
$$D = 1.417, p_0^{\text{emp}} = 0.9298$$

## 4.3 Fitting Models

[2], [3], [4], [5], [6] ABM($r = 9$), [7] LMS ($r = 5$), and [8] LMNS($r = 4$).

| # of claims | frequency | [2] | [3] | [4] | [5] | [6] | [7] | [8] |
|---|---|---|---|---|---|---|---|---|
| 0 | 3719 | 3718.58 | 3676.2 | 3719.06 | 3718.30 | 3718.98 | 3719.65 | 3718.83 |
| 1 | 232 | 234.54 | 302.4 | 228.65 | 234.01 | 232.18 | 231.08 | 233.19 |
| 2 | 38 | 34.86 | 20.1 | 41.85 | 36.09 | 37.29 | 37.57 | 36.30 |
| 3 | 7 | 8.32 | 1.2 | 8.32 | 8.13 | 8.36 | 8.48 | 8.28 |
| 4 | 3 | 2.45 | 0.1 | 1.68 | 2.26 | 2.22 | 2.25 | 2.30 |
| 5 | 1 | 0.80 | 0.0 | 0.40 | 0.72 | 0.65 | 0.66 | 0.72 |
| $L$ | | -1183.52 | -1217.70 | -1183.97 | -1183.44 | -1183.37 | **-1183.36** | -1183.41 |
| $\chi^2$ | | 0.5438 | 106.5 | 2.312 | 0.6240 | 0.4481 | 0.4555 | 0.3827 |
| df | | 2 | 3 | 2 | 2 | 2 | 1 | 2 |
| $p$-value | | 0.7619 | 0.0 | 0.3147 | 0.7320 | 0.7993 | 0.4997 | **0.8258** |
| RMSE | | 1.760 | 34.55 | 2.235 | 1.296 | **0.7212** | 0.8470 | 1.043 |

# 5 Data Set 5

Automobile claim data in Belgium 1975-1976, see [1].

| value | 0 | 1 | 2 | 3 | 4 |
|---|---|---|---|---|---|
| frequency | 96978 | 9240 | 704 | 43 | 9 |

## 5.1 Literature


[1] Gossiaux, A. and Lemaire, J. (1981). Methodes d'ajustement de distributions de sinistres. *Bulletin of the Association of Swiss Actuaries* 81, 87-95.

[2] Willmot, G. (1987). The Poisson-Inverse Gaussian distribution as an alternative to the negative binomial. *Scandinavian Actuarial Journal* 3-4, 113-127.

[3] Gomez-Deniz, E. and Calderin-Ojeda, E. (2011a). The discrete Lindley distribution: properties and applications. *Journal of Statistical Computation and Simulation* 81, 1405-1416.


## 5.2 Descriptive Statistics

$$\overline{x} = 0.1011,\ s^2 = 0.1074,\ b_1 = 3.454,$$
$$D = 1.063, p_0^{\text{emp}} = 0.9066$$

## 5.3 Fitting Models

[2], [3], [4] ABM($r = 9$) , [5] LMS($r = 2$), and [6] LMNS($r = 1$).

| # of claims | frequency | [2] | [3] | [4] | [5] | [6] |
|---|---|---|---|---|---|---|
| 0 | 96978 | 96978.53 | 96981.05 | 96980.18 | 96980.54 | 96978.53 |
| 1 | 9240 | 9230.90 | 9229.71 | 9234.52 | 9233.26 | 9240.56 |
| 2 | 704 | 697.63 | 710.16 | 703.80 | 705.13 | 697.43 |
| 3 | 43 | 52.85 | 49.58 | 51.42 | 51.12 | 52.80 |
| 4 | 9 | 4.21 | 3.27 | 3.77 | 3.67 | 4.27 |
| $L$ | | -36103.6 | -36104.2 | -36103.8 | -36103.8 | **-36103.5** |
| $\chi^2$ | | 6.119 | 9.610 | 7.353 | 7.725 | 5.871 |
| df | | 2 | 3 | 2 | 1 | 2 |
| $p$-value | | 0.04692 | 0.02219 | 0.02531 | $< 0.01$ | **0.05309** |
| RMSE | | 5.675 | 6.771 | **5.159** | 5.431 | 5.698 |

# 6 Data Set 6

Insurance claims in Germany in 1960, see [1].

| value | 0 | 1 | 2 | 3 | 4 | 5 | 6 |
|---|---|---|---|---|---|---|---|
| frequency | 20592 | 2651 | 297 | 41 | 7 | 0 | 1 |

## 6.1 Literature


[1] Gossiaux, A. and Lemaire, J. (1981). Methodes d'ajustement de distributions de sinistres. *Bulletin of the Association of Swiss Actuaries* 81, 87-95.

[2] Willmot, G. (1987). The Poisson-Inverse Gaussian distribution as an alternative to the negative binomial. *Scandinavian Actuarial Journal* 3-4, 113-127.

[3] Gomez-Deniz, E. and Calderin-Ojeda, E. (2011a). The discrete Lindley distribution: properties and applications. *Journal of Statistical Computation and Simulation* 81, 1405-1416.

[4] Kokonendji, C.C. and M. Khoudar (2004a). On strict arcsine distribution. *Communications in Statistics - Theory and Methods* 33(5), 993-1006.


## 6.2 Descriptive Statistics

$$\overline{x} = 0.1442,\ s^2 = 0.1639,\ b_1 = 3.230,$$
$$D = 1.136, p_0^{\text{emp}} = 0.8729$$

## 6.3 Fitting Models

[2], [3], [4], [5] ABM($r = 9$), [6] LMS ($r = 3$), and [7] LMNS($r = 1$).

| # of claims | frequency | [2] | [3] | [4] | [5] | [6] | [7] |
|---|---|---|---|---|---|---|---|
| 0 | 20592 | 20595.74 | 20544.79 | 20685.83 | 20596.75 | 20598.34 | 20595.56 |
| 1 | 2651 | 2638.81 | 2720.36 | 2663.08 | 2633.91 | 2630.78 | 2639.47 |
| 2 | 297 | 308.08 | 292.41 | 171.42 | 313.69 | 315.12 | 307.61 |
| 3 | 41 | 39.68 | 28.55 | 55.00 | 38.81 | 38.97 | 39.50 |
| 4 | 7 | 5.65 | 2.64 | 9.62 | 5.04 | 5.02 | 5.73 |
| 5 | 0 | 0.87 | 0.24 | 3.24 | 0.68 | 0.67 | 0.93 |
| 6 | 1 | 0.14 | 0.02 | 0.54 | 0.10 | 0.09 | 0.16 |
| $L$ | | -10221.87 | -10228.45 | -10263.11 | -10222.51 | -10222.64 | **-10221.78** |
| $\chi^2$ | | 0.7588 | 16.38 | 98.33 | 1.924 | 2.146 | 0.6649 |
| df | | 2 | 3 | 2 | 2 | 1 | 2 |
| $p$-value | | 0.6843 | $< 0.001$ | 0.0 | 0.3821 | 0.1430 | **0.7172** |
| RMSE | | 6.442 | 32.15 | 59.68 | 9.282 | 10.60 | **6.136** |

# 7 Data Set 7

The number of European red mites on apple leaves, see [1].

| value | 0 | 1 | 2 | 3 | 4 | 5 | 6 | 7 | 8 |
|---|---|---|---|---|---|---|---|---|---|
| frequency | 70 | 38 | 17 | 10 | 9 | 3 | 2 | 1 | 0 |

## 7.1 Literature

[1] Bliss, C.I. and R.A. Fisher (1953). Fitting the negative binomial distribution to biological data. *Biometrics* 9(2), 176-200.

[2] Chakraborty, S. and D. Chakravarty (2012). Discrete Gamma Distributions: Properties and Parameter Estimations. *Communications in Statistics - Theory and Methods* 41(18), 3301-3324.

[3] Alamatsaz, M.H., S. Deey, T. Dey, and S. Shams Harandi (2016). Discrete generalized Rayleigh distribution. *Pakistan Journal of Statistics* 32(1), 1-20.

## 7.2 Descriptive Statistics

$$\overline{x} = 1.147,\ s^2 = 2.274,\ b_1 = 1.514$$
$$D = 1.983, p_0^{\text{emp}} = 0.4666$$

## 7.3 Fitting Models

[2], [3], [4] ABM($r = 2$), [5] LMS ($r = 1$), and [6] LMNS($r = 9$).

| # of red mites | frequency | [2] | [3] | [4] | [5] | [6] |
|---|---|---|---|---|---|---|
| 0 | 70 | 69.67 | 71.09 | 68.85 | 69.25 | 67.89 |
| 1 | 38 | 37.49 | 32.08 | 38.90 | 38.20 | 40.51 |
| 2 | 17 | 20.02 | 20.76 | 20.04 | 20.04 | 20.19 |
| 3 | 10 | 10.67 | 12.88 | 10.35 | 10.50 | 10.00 |
| 4 | 9 | 5.69 | 7.25 | 5.43 | 5.55 | 5.11 |
| 5 | 3 | 3.03 | 3.60 | 2.90 | 2.69 | 2.71 |
| 6 | 2 | 1.61 | 1.54 | 1.57 | 1.59 | 1.49 |
| 7 | 1 | 0.86 | 0.56 | 0.86 | 0.86 | 0.84 |
| 8 | 0 | 0.96 | | 0.48 | 0.47 | 0.49 |
| $L$ | | -222.44 | **-221.24** | -222.75 | -222.59 | -223.29 |
| $\chi^2$ | | 2.896 | 2.868 | 3.461 | 3.180 | 4.483 |
| df | | 5 | 5 | 5 | 4 | 5 |
| $p$-value | | 0.7160 | **0.7204** | 0.6293 | 0.5281 | 0.4821 |
| RMSE | | **1.563** | 2.635 | 1.656 | 1.578 | 2.018 |

# 8 Data Set 8

The number of accidents experienced by machinists, see [1].

| value | 0 | 1 | 2 | 3 | 4 | 5 | 6 | 7 | 8 |
|---|---|---|---|---|---|---|---|---|---|
| frequency | 296 | 74 | 26 | 8 | 4 | 4 | 1 | 0 | 1 |

## 8.1 Literature

[1] Bliss, C.I. and R.A. Fisher (1953). Fitting the negative binomial distribution to biological data. *Biometrics* 9(2), 176-200.

[2] Bhati, D. and H.S. Bakouch (2019). A new infinitely divisible discrete distribution with applications to count data modeling. *Communications in Statistics - Theory and Methods* 48(6), 1401-1416.

### 8.2 Descriptive Statistics

$$\overline{x} = 0.4831,\ s^2 = 1.011,\ b_1 = 3.163$$
$$D = 2.092, p_0^{\text{emp}} = 0.7150$$

### 8.3 Fitting Models

[2], [3] ABM($r = 9$), [4] LMS ($r = 4$), and [5] LMNS($r = 3$).

| # of accidents | frequency | [1] | [2] | [3] | [4] |
|---:|---:|---:|---:|---:|---:|
| 0 | 296 | 296.60 | 295.91 | 296.44 | 295.30 |
| 1 | 74 | 72.34 | 74.37 | 73.61 | 76.23 |
| 2 | 26 | 25.48 | 24.80 | 24.83 | 24.20 |
| 3 | 8 | 10.47 | 9.90 | 10.00 | 9.37 |
| 4 | 4 | 4.68 | 4.43 | 4.50 | 4.18 |
| 5 | 4 | 2.21 | 2.14 | 2.18 | 2.06 |
| 6 | 1 | | 1.10 | 1.11 | 1.09 |
| 7 | 0 | 2.21 | 0.58 | 0.59 | 0.61 |
| 8 | 1 | | 0.32 | 0.32 | 0.36 |
| $L$ | | -381.82 | -381.80 | **-381.78** | -381.95 |
| $\chi^2$ | | 2.205 | 0.8985 | 0.9239 | 0.7534 |
| df | | 3 | 3 | 2 | 3 |
| $p$-value | | 0.820 | 0.8258 | 0.6300 | **0.8606** |
| RMSE | | 1.373 | **1.035** | 1.060 | 1.297 |

# 9 Data Set 9

The number of hospitalizations per family per year, see [1].

| value | 0 | 1 | 2 | 3 | 4 |
|---|---|---|---|---|---|
| frequency | 2659 | 244 | 19 | 2 | 0 |

### 9.1 Literature


[1] Klugman, S., H. Panjer, and G. Willmot (2008). *Loss Models. From Data to Decisions.* 3-rd Edition, John Wiley and Sons, New York.

[2] Gomez-Deniz, E., J.M. Sarabia, and E. Calderin-Ojeda (2011b). A new discrete distribution with actuarial applications. *Insurance: Mathematics and Economics* 48(3), 406-412.


### 9.2 Descriptive Statistics

$$\overline{x} = 0.09850,\ s^2 = 0.1059,\ b_1 = 3.529,$$
$$D = 1.075, p_0^{\text{emp}} = 0.9094$$

### 9.3 Fitting Models

[2], [3] ABM($r = 9$), [4] LMS ($r = 3$), and [5] LMNS($r = 1$).

| # of hospitalizations | frequency | [2] | [3] | [4] | [5] |
|---:|---:|---:|---:|---:|---:|
| 0 | 2659 | 2659.02 | 2659.03 | 2659.03 | 2658.95 |
| 1 | 244 | 243.79 | 243.80 | 243.78 | 244.05 |
| 2 | 19 | 19.52 | 19.47 | 19.50 | 19.22 |
| 3 | 2 | 1.54 | 1.56 | 1.55 | 1.61 |
| 4+ | 0 | 0.11 | 0.13 | 0.13 | 0.15 |
| $L$ | | **-969.06** | **-969.06** | **-969.06** | -969.07 |
| $\chi^2$ | | 0.0765 | 0.0634 | 0.2786 | 0.03196 |
| df | | 1 | 1 | 1 | 1 |
| $p$-value | | 0.7821 | 0.8011 | 0.5976 | **0.8581** |
| RMSE | | 0.3278 | 0.3060 | 0.3205 | **0.2153** |

## 10 Data Set 10

Number of claims of automobile liability policies, see [1].

| value | 0 | 1 | 2 | 3 | 4 | 5 | 6 | 7 | 8 | 9 | 10 | 11 | 12 |
|---|---|---|---|---|---|---|---|---|---|---|---|---|---|
| frequency | 99 | 65 | 57 | 35 | 20 | 10 | 4 | 0 | 3 | 4 | 0 | 1 | 0 |

### 10.1 Literature


[1] Klugman, S., H. Panjer, and G. Willmot (2008). *Loss Models. From Data to Decisions.* 3-rd Edition, John Wiley and Sons, New York.

[2] Gomez-Deniz, E., J.M. Sarabia, and E. Calderin-Ojeda (2011b). A new discrete distribution with actuarial applications. *Insurance: Mathematics and Economics* 48(3), 406-412.


### 10.2 Descriptive Statistics

$$\overline{x} = 1.708,\ s^2 = 3.669,\ b_1 = 1.707$$
$$D = 2.148, p_0^{\text{emp}} = 0.3322$$

### 10.3 Fitting Models

[2], [3] ABM($r = 2$) , [4] LMS($r = 1$), and [5] LMNS($r = 9$).

| # of claims | frequency | [2] | [3] | [4] | [5] |
|---|---|---|---|---|---|
| 0 | 99 | 96.57 | 94.11 | 95.02 | 91.76 |
| 1 | 65 | 73.26 | 78.36 | 77.13 | 81.24 |
| 2 | 57 | 50.79 | 51.03 | 50.68 | 52.26 |
| 3 | 35 | 32.48 | 30.87 | 31.05 | 30.61 |
| 4 | 20 | 19.54 | 18.18 | 18.45 | 17.50 |
| 5 | 10 | 11.27 | 10.60 | 10.80 | 10.02 |
| 6 | 4 | 6.33 | 6.17 | 6.27 | 5.81 |
| 7 | 0 | 3.50 | 3.59 | 3.63 | 3.42 |
| 8 | 3 | 1.92 | 2.10 | 2.10 | 2.04 |
| 9 | 4 | 1.05 | 1.23 | 1.21 | 1.24 |
| 10 | 0 | 0.57 | 0.72 | 0.70 | 0.77 |
| 11 | 1 | 0.31 | 0.43 | 0.40 | 0.48 |
| 12 | 0 | 0.17 | 0.25 | 0.23 | 0.30 |
| $L$ | | **-528.4** | -529.1 | -528.9 | -529.7 |
| $\chi^2$ | | 2.408 | 4.815 | 4.815 | 5.871 |
| df | | 4 | 5 | 4 | 5 |
| $p$-value | | **0.6612** | 0.4388 | 0.3524 | 0.3189 |
| RMSE | | **3.3894** | 4.689 | 4.379 | 5.466 |

# 11 Data Set 11

Automobile claim data in Central African Republic 1984, see [1].

| value | 0 | 1 | 2 | 3 | 4 | 5+ |
|---|---|---|---|---|---|---|
| frequency | 6984 | 2452 | 433 | 100 | 26 | 5 |

## 11.1 Literature


[1] Kokonendji, C.C. and M. Khoudar (2004a). On strict arcsine distribution. *Communications in Statistics - Theory and Methods* 33(5), 993-1006.


## 11.2 Descriptive Statistics

$$\overline{x} = 0.3747,\ s^2 = 0.4221,\ b_1 = 2.054$$
$$D = 1.127, p_0^{\mathrm{emp}} = 0.6984$$

## 11.3 Fitting Models

[1], [2] ABM($r = 9$) , [3] LMS($r = 3$), and [4] LMNS($r = 1$).

| # of claims | frequency | [1] | [2] | [3] | [4] |
|---|---|---|---|---|---|
| 0 | 6984 | 7012.25 | 7015.68 | 7023.47 | 7017.65 |
| 1 | 2452 | 2461.02 | 2356.66 | 2344.67 | 2356.43 |
| 2 | 433 | 431.77 | 514.86 | 516.49 | 511.40 |
| 3 | 100 | 76.24 | 94.11 | 95.89 | 94.53 |
| 4 | 26 | 16.16 | 15.73 | 16.33 | 16.51 |
| $\geq 5$ | 5 | 2.56 | 2.51 | 2.65 | 2.86 |
| $L$ | | **-7973.3** | -7979.7 | -7979.9 | -7978.5 |
| $\chi^2$ | | 15.61 | 25.48 | 25.62 | 22.45 |
| df | | 2 | 2 | 1 | 2 |
| $p$-value | | **0.0004** | 0.0 | 0.0 | 0.0 |
| RMSE | | **16.06** | 53.14 | 57.97 | 52.50 |

# 12 Data Set 12

The length of stays (LoS) after hospital admission in the USA among the elderly population, aged 65 years or more, see [1].

| value | 0 | 1 | 2 | 3 | 4 | 5 | 6 | 7 | 8 |
|---|---|---|---|---|---|---|---|---|---|
| frequency | 3541 | 599 | 176 | 48 | 20 | 12 | 5 | 1 | 4 |

## 12.1 Literature


[1] Deb, P. and P.K. Trivedi (1997). Demand for Medical Care by the Elderly: A Finite Mixture Approach. *Journal of Applied Econometrics* 12(3), 313-336.

[2] Bhati, D. and H.S. Bakouch (2019). A new infinitely divisible discrete distribution with applications to count data modeling. *Communications in Statistics - Theory and Methods* 48(6), 1401-1416.


## 12.2 Descriptive Statistics

$$\overline{x} = 0.2960,\ s^2 = 0.5571,\ b_1 = 3.963$$
$$D = 1.882, p_0^{\text{emp}} = 0.8038$$

## 12.3 Fitting Models

[2], [3] ABM($r = 9$) , [4] LMS($r = 4$), and [5] LMNS($r = 9$).

| LoS | frequency | [2] | [3] | [4] | [5] |
|---|---|---|---|---|---|
| 0 | 3541 | 3543.51 | 3540.84 | 3541.38 | 3539.48 |
| 1 | 599 | 595.78 | 602.44 | 600.34 | 607.65 |
| 2 | 176 | 167.26 | 164.57 | 165.73 | 161.79 |
| 3 | 48 | 58.36 | 56.93 | 57.49 | 55.50 |
| 4 | 20 | 22.98 | 22.57 | 22.70 | 22.19 |
| 5 | 12 | 9.76 | 9.77 | 9.74 | 9.80 |
| 6 | 5 | 4.37 | 4.49 | 4.42 | 4.64 |
| 7 | 1 | 3.98 | 2.16 | 2.09 | 2.31 |
| 8 | 4 | | 1.07 | 1.02 | 1.20 |
| $L$ | | -3007.6 | **-3007.4** | -3007.5 | -3007.5 |
| $\chi^2$ | | 3.564 | 3.154 | 3.287 | 3.124 |
| df | | 5 | 5 | 4 | 5 |
| $p$-value | | 0.614 | 0.6762 | 0.5110 | **0.6809** |
| RMSE | | 5.158 | 5.205 | **4.9486** | 6.278 |

# 13 Data Set 13

The number of carious teeth among the four deciduous molars in a sample of 100 children aged 10 and 11 years, see [1].

| value | 0 | 1 | 2 | 3 | 4+ |
|---|---|---|---|---|---|
| frequency | 64 | 17 | 10 | 6 | 3 |

## 13.1 Literature


[1] Krishna, H. and P.S. Pundir (2009). Discrete Burr and discrete Pareto distributions. *Statistical Methodology* 6, 177–188.

[2] El-Morshedy, M., M.S. Eliwa, and H. Nagy (2020). A new two-parameter exponentiated discrete Lindley distribution: properties, estimation and applications. *Journal of Applied Statistics* 47(2), 354-375.


## 13.2 Descriptive Statistics

$$\overline{x} = 0.67,\ s^2 = 1.153,\ b_1 = 1.548$$
$$D = 1.720, p_0^{\text{emp}} = 0.64$$

## 13.3 Fitting Models

[2], [3] ABM($r = 2$) , [4] LMS($r = 1$), and [5] LMNS($r = 9$).

| # of cases | frequency | [2] | [3] | [4] | [5] |
|---|---|---|---|---|---|
| 0 | 64 | 63.57 | 62.40 | 62.79 | 61.80 |
| 1 | 17 | 19.75 | 21.88 | 21.33 | 22.89 |
| 2 | 10 | 9.09 | 8.66 | 8.67 | 8.58 |
| 3 | 6 | 4.19 | 3.73 | 3.81 | 3.53 |
| $\geq 4$ | 3 | 3.4 | 1.70 | 1.75 | 1.58 |
| $L$ | | **-111.45** | -112.4 | -112.2 | -112.9 |
| $\chi^2$ | | 0.739 | 1.874 | 2.406 | 2.597 |
| df | | 1 | 1 | 1 | 1 |
| $p$-value | | **0.390** | 0.1711 | 0.1209 | 0.1071 |
| RMSE | | **1.549** | 2.647 | 2.378 | 3.151 |

# 14 Data Set 14

The counts of cysts of kidneys using steroids, see [1].

| value | 0 | 1 | 2 | 3 | 4 | 5 | 6 | 7 | 8 | 9 | 10 | 11 |
|---|---|---|---|---|---|---|---|---|---|---|---|---|
| frequency | 65 | 14 | 10 | 6 | 4 | 2 | 2 | 2 | 1 | 1 | 1 | 2 |

## 14.1 Literature


[1] Chan, S., P.R. Riley, K.L. Price, F. McElduff, and P.J. Winyard (2009). Corticosteroid-induced kidney dysmorphogenesis is associated with deregulated expression of known cyst genic molecules, as well as Indian hedgehog. *American Journal of Physiology Tenal Physiology* 298(2), 346-356.

[2] El-Morshedy, M., M.S. Eliwa, and H. Nagy (2020). A new two-parameter exponentiated discrete Lindley distribution: properties, estimation and applications. *Journal of Applied Statistics* 47(2), 354-375.


## 14.2 Descriptive Statistics

$$\overline{x} = 1.391,\ s^2 = 6.112,\ b_1 = 2.230$$
$$D = 4.394, p_0^{\text{emp}} = 0.5909$$

## 14.3 Fitting Models

[2], [3] ABM($r = 2$) , [4] LMS($r = 1$), and [5] LMNS($r = 9$).

| # of cysts | frequency | [2] | [3] | [4] | [5] |
|---|---|---|---|---|---|
| 0 | 65 | 64.97 | 63.20 | 63.95 | 61.46 |
| 1 | 14 | 14.39 | 19.19 | 17.93 | 22.40 |
| 2 | 10 | 9.01 | 9.24 | 9.10 | 9.86 |
| 3 | 6 | 6.14 | 5.34 | 5.47 | 5.14 |
| 4 | 4 | 4.33 | 3.41 | 3.57 | 3.02 |
| 5 | 2 | 3.10 | 2.32 | 2.46 | 1.93 |
| 6 | 2 | 2.24 | 1.65 | 1.76 | 1.32 |
| 7 | 2 | 1.62 | 1.21 | 1.29 | 0.94 |
| 8 | 1 | 1.18 | 0.91 | 0.96 | 0.70 |
| 9 | 1 | 0.85 | 0.69 | 0.73 | 0.53 |
| 10 | 1 | 0.62 | 0.54 | 0.56 | 0.41 |
| 11 | 2 | 0.44 | 0.42 | 0.44 | 0.33 |
| $L$ | | **-166.9** | -168.7 | -168.1 | -171.1 |
| $\chi^2$ | | 0.6513 | 2.145 | 1.445 | 5.091 |
| df | | 4 | 4 | 3 | 4 |
| $p$-value | | **0.9572** | 0.7090 | 0.6949 | 0.2781 |
| RMSE | | **0.6653** | 1.713 | 1.332 | 2.737 |

# Part II
# Comparison with Selected Distributions

In the second part we compare our two-parameter models ABM and LMNS with the Poisson-inverse Gaussian (PIG), the new logarithmic distribution (NLD), and the exponentiated dicrete Lindley distribution (EDLID), see [1], [2], and [3]. All these have two parameters which are estimated by the maximum likelihood method.


[1] Willmot, G. (1987). The Poisson-Inverse Gaussian distribution as an alternative to the negative binomial. *Scandinavian Actuarial Journal* 3-4, 113-127.

[2] Gomez-Deniz, E., J.M. Sarabia, and E. Calderin-Ojeda (2011b). A new discrete distribution with actuarial applications. *Insurance: Mathematics and Economics* 48(3), 406-412.

[3] El-Morshedy, M., M.S. Eliwa, and H. Nagy (2020). A new two-parameter exponentiated discrete Lindley distribution: properties, estimation and applications. *Journal of Applied Statistics* 47(2), 354-375.


## 15 Comparison

First the same 14 data sets of Part I, and then some others. We just report the log likelihood, the $\chi^2$-value, the $p$-value, and the root mean square error (rmse).

1.

| value | 0 | 1 | 2 | 3 | 4 | 5 | 6 |
|---|---|---|---|---|---|---|---|
| frequency | 103704 | 14075 | 1766 | 255 | 45 | 6 | 2 |

| | PIG | NLD | EDLID | ABM | LMNS |
|---|---|---|---|---|---|
| $L$ | -54609.76 | -54615.06 | -54621.37 | -54611.59 | **-54609.75** |
| $\chi^2$ | 0.7783 | 11.94 | 26.57 | 4.477 | **0.7432** |
| $p$-value | 0.8546 | 0.007592 | 0.0 | 0.2143 | **0.8630** |
| RMSE | 10.89 | 39.98 | 55.54 | 31.75 | **8.182** |

2.

| value | 0 | 1 | 2 | 3 | 4 | 5 |
|---|---|---|---|---|---|---|
| frequency | 370412 | 46545 | 3935 | 317 | 28 | 3 |

| | PIG | NLD | EDLID | ABM | LMNS |
|---|---|---|---|---|---|
| $L$ | -171134.47 | **-171133.30** | -171134.58 | -171135.5 | 171134.40 |
| $\chi^2$ | 2.744 | **0.3709** | 2.979 | 5.168 | 2.605 |
| $p$-value | 0.2536 | **0.8307** | 0.2254 | 0.07548 | 0.2718 |
| RMSE | 38.84 | **4.278** | 22.46 | 49.37 | 38.36 |

3.

| value | 0 | 1 | 2 | 3 | 4 | 5 | 6 | 7 |
|---|---|---|---|---|---|---|---|---|
| frequency | 7840 | 1317 | 239 | 42 | 14 | 4 | 4 | 1 |

| | PIG | NLD | EDLID | ABM | LMNS |
|---|---|---|---|---|---|
| $L$ | 5343.51 | -5349.07 | -5352.76 | -5345.04 | **-5342.89** |
| $\chi^2$ | 4.536 | 17.77 | 29.07 | . 7.750 | **3.375** |
| $p$-value | 0.2091 | $< 0.001$ | 0.0 | . 0.05148 | **0.3374** |
| RMSE | 5.814 | 12.07 | 15.05 | . 9.415 | **4.962** |

4.

| value | 0 | 1 | 2 | 3 | 4 | 5 |
|---|---|---|---|---|---|---|
| frequency | 3719 | 232 | 38 | 7 | 3 | 1 |

| | PIG | NLD | EDLID | ABM | LMNS |
|---|---|---|---|---|---|
| $L$ | -1183.52 | -1183.97 | -1184.48 | **-1183.37** | -1183.41 |
| $\chi^2$ | 0.5438 | 2.312 | 3.652 | 0.4481 | **0.3827** |
| $p$-value | 0.7619 | 0.3147 | 0.1611 | 0.7993 | **0.8258** |
| RMSE | 1.760 | 2.235 | 3.001 | **0.7212** | 1.043 |

5.

| value | 0 | 1 | 2 | 3 | 4 |
|---|---|---|---|---|---|
| frequency | 96978 | 9240 | 704 | 43 | 9 |

| | PIG | NLD | EDLID | ABM | LMNS |
|---|---|---|---|---|---|
| $L$ | -36103.57 | -36103.76 | -36104.21 | -36103.77 | **-36103.53** |
| $\chi^2$ | 6.119 | 7.204 | 9.700 | 7.353 | **5.871** |
| $p$-value | 0.04692 | 0.02727 | $< 0.01$ | 0.02531 | **0.05309** |
| RMSE | 5.675 | 4.917 | **4.795** | 5.159 | 5.698 |

6.

| value | 0 | 1 | 2 | 3 | 4 | 5 | 6 |
|---|---|---|---|---|---|---|---|
| frequency | 20592 | 2651 | 297 | 41 | 7 | 0 | 1 |

| | PIG | NLD | EDLID | ABM | LMNS |
|---|---|---|---|---|---|
| $L$ | -10221.87 | -10223.22 | -10224.54 | -10222.51 | **-10221.78** |
| $\chi^2$ | 0.7588 | 3.251 | 5.961 | 1.924 | **0.6649** |
| $p$-value | 0.6843 | 0.1969 | 0.05078 | 0.3821 | **0.7172** |
| RMSE | 6.442 | 8.944 | 11.18 | 9.282 | **6.136** |

7.

| value | 0 | 1 | 2 | 3 | 4 | 5 | 6 | 7 | 8 |
|---|---|---|---|---|---|---|---|---|---|
| frequency | 70 | 38 | 17 | 10 | 9 | 3 | 2 | 1 | 0 |

| | PIG | NLD | EDLID | ABM | LMNS |
|---|---|---|---|---|---|
| $L$ | -223.51 | -222.44 | **-222.27** | -222.75 | -223.29 |
| $\chi^2$ | 4.935 | 2.918 | **2.672** | 3.461 | 4.483 |
| $p$-value | 0.4239 | 0.7126 | **0.7504** | 0.6293 | 0.4821 |
| RMSE | 2.184 | **1.562** | 1.725 | 1.656 | 2.018 |

8.

| value | 0 | 1 | 2 | 3 | 4 | 5 | 6 | 7 | 8 |
|---|---|---|---|---|---|---|---|---|---|
| frequency | 296 | 74 | 26 | 8 | 4 | 4 | 1 | 0 | 1 |

| | PIG | NLD | EDLID | ABM | LMNS |
|---|---|---|---|---|---|
| $L$ | -381.92 | -382.13 | -382.97 | **-381.80** | -381.95 |
| $\chi^2$ | 0.7901 | 2.293 | 4.199 | 0.8985 | **0.7534** |
| $p$-value | 0.8518 | 0.5139 | 0.2408 | 0.8258 | **0.8606** |
| RMSE | 1.506 | 1.732 | 2.585 | **1.035** | 1.297 |

9.

| value | 0 | 1 | 2 | 3 | 4 |
|---|---|---|---|---|---|
| frequency | 2659 | 244 | 19 | 2 | 0 |

| | PIG | NLD | EDLID | ABM | LMNS |
|---|---|---|---|---|---|
| $L$ | -969.07 | **-969.06** | -969.07 | -969.06 | -969.07 |
| $\chi^2$ | 0.03206 | 0.0765 | 0.1478 | 0.06344 | **0.03196** |
| $p$-value | 0.8579 | 0.7821 | 0.7007 | 0.8011 | **0.8581** |
| RMSE | 0.2155 | 0.3278 | 0.4461 | 0.3060 | **0.2153** |

10.

| value | 0 | 1 | 2 | 3 | 4 | 5 | 6 | 7 | 8 | 9 | 10 | 11 | 12 |
|---|---|---|---|---|---|---|---|---|---|---|---|---|---|
| frequency | 99 | 65 | 57 | 35 | 20 | 10 | 4 | 0 | 3 | 4 | 0 | 1 | 0 |

| | PIG | NLD | EDLID | ABM | LMNS |
|---|---|---|---|---|---|
| $L$ | -530.10 | **-528.40** | -528.56 | -529.08 | -529.66 |
| $\chi^2$ | 6.798 | **2.971** | 3.495 | 4.815 | 5.871 |
| $p$-value | 0.2361 | **0.7043** | 0.6241 | 0.4388 | 0.3189 |
| RMSE | 5.952 | **3.389** | 3.588 | 4.689 | 5.466 |

11.

| value | 0 | 1 | 2 | 3 | 4 | 5+ |
|---|---|---|---|---|---|---|
| frequency | 6984 | 2452 | 433 | 100 | 26 | 5 |

| | PIG | NLD | EDLID | ABM | LMNS |
|---|---|---|---|---|---|
| $L$ | -7978.60 | -7977.27 | **-7976.19** | -7979.71 | -7978.53 |
| $\chi^2$ | 22.73 | 20.62 | **18.93** | 25.49 | 22.50 |
| $p$-value | 4.6e-05 | 1.3e-04 | **2.8e-04** | 1.2e-05 | 5.1e-05 |
| RMSE | 52.64 | 40.78 | **32.75** | 53.14 | 52.50 |

12.

| value | 0 | 1 | 2 | 3 | 4 | 5 | 6 | 7 | 8 |
|---|---|---|---|---|---|---|---|---|---|
| frequency | 3541 | 599 | 176 | 48 | 20 | 12 | 5 | 1 | 4 |

| | PIG | NLD | EDLID | ABM | LMNS |
|---|---|---|---|---|---|
| $L$ | -3008.24 | -3011.44 | -3016.51 | **-3007.43** | -3007.48 |
| $\chi^2$ | 4.715 | 12.80 | 27.40 | 3.154 | **3.124** |
| $p$-value | 0.4517 | 0.02534 | 0.0. | 0.6762 | **0.6809** |
| RMSE | 9.994 | 9.005 | 13.88 | **5.205** | 6.278 |

13.

| value | 0 | 1 | 2 | 3 | 4+ |
|---|---|---|---|---|---|
| frequency | 64 | 17 | 10 | 6 | 3 |

| | PIG | NLD | EDLID | ABM | LMNS |
|---|---|---|---|---|---|
| $L$ | -113.24 | -112.01 | **-111.45** | -112.43 | -112.92 |
| $\chi^2$ | 3.046 | 1.353 | **0.7438** | 1.874 | 2.597 |
| $p$-value | 0.08095 | 0.2447 | **0.3884** | 0.1711 | 0.1071 |
| RMSE | 3.445 | 2.186 | **1.616** | 2.647 | 3.151 |

14.

| value | 0 | 1 | 2 | 3 | 4 | 5 | 6 | 7 | 8 | 9 | 10 | 11 |
|---|---|---|---|---|---|---|---|---|---|---|---|---|
| frequency | 65 | 14 | 10 | 6 | 4 | 2 | 2 | 2 | 1 | 1 | 1 | 2 |

| | PIG | NLD | EDLID | ABM | LMNS |
|---|---|---|---|---|---|
| $L$ | -170.87 | -167.52 | **-166.95** | -168.73 | -171.06 |
| $\chi^2$ | 4.902 | 1.024 | **0.6513** | 2.145 | 5.091 |
| $p$-value | 0.2975 | 0.9061 | **0.9572** | 0.7090 | 0.2781 |
| RMSE | 2.763 | 1.039 | **0.6653** | 1.713 | 2.737 |

15. The number of accidents of workers in a particular division of a large steel corporation in an observational period of six months.

Sichel, H. S. (1951). The estimation of the parameters of a negative binomial distribution with special reference to psychological data. *Psychometrika* 16(1), 107– 27.

| value | 0 | 1 | 2 | 3 | 4 | 5 | 6 |
|---|---|---|---|---|---|---|---|
| frequency | 217 | 44 | 29 | 11 | 11 | 2 | 4 |

$$\overline{x} = 0.6698,\ s^2 = 1.534,\ b_1 = 2.181,$$
$$D = 2.290, p_0^{\text{emp}} = 0.6824$$

| | PIG | NLD | EDLID | ABM | LMNS |
|---|---|---|---|---|---|
| $L$ | -352.69 | -347.70 | **-346.21** | -349.50 | -351.73 |
| $\chi^2$ | 15.82 | 6.892 | **4.338** | 9.884 | 13.92 |
| df | 3 | 3 | 3 | 3 | 3 |
| $p$-value | $< 0.01$ | 0.07541 | **0.2272** | 0.01958 | $< 0.01$ |
| RMSE | 8.206 | 4.453 | **3.258** | 5.898 | . 7.516 |

16. The number of chromatid aberrations in 24 hours.

Catcheside, D.G., D.E. Lea, and J.M. Thoday (1946). Types of chromosome structural change induced by the irradiation of Tradescantia microspores. *Journal of Genetics* 47(2), 113–36.

| value | 0 | 1 | 2 | 3 | 4 | 5 | 6 | 7 |
|---|---|---|---|---|---|---|---|---|
| frequency | 268 | 87 | 26 | 9 | 4 | 2 | 1 | 1 |

$$\overline{x} = 0.5475,\ s^2 = 1.126,\ b_1 = 3.110$$
$$D = 2.056, p_0^{\text{emp}} = 0.67$$

| | PIG | NLD | EDLID | ABM | LMNS |
|---|---|---|---|---|---|
| $L$ | **-398.40** | -399.99 | -401.47 | -398.82 | -398.50 |
| $\chi^2$ | 0.7603 | 3.684 | 6.122 | 1.608 | **0.4372** |
| df | 3 | 3 | 3 | 3 | 3 |
| $p$-value | 0.8589 | 0.2976 | 0.1058 | 0.6575 | **0.9325** |
| RMSE | 1.717 | 3.679 | 4.514 | 2.578 | **1.161** |

17. The number of women who are working on shells for 5 weeks.

Consul, P.C. and G.G. Jain (1973). A generalization of the Poisson distribution. *Technometrics* 15(4), 791-799.

| value | 0 | 1 | 2 | 3 | 4 | 5+ |
|---|---|---|---|---|---|---|
| frequency | 447 | 132 | 42 | 21 | 3 | 2 |

$\overline{x} = 0.4652,\ s^2 = 0.6919,\ b_1 = 2.116$
$D = 1.487, p_0^{\text{emp}} = 0.6909$

| | PIG | NLD | EDLID | ABM | LMNS |
|---|---|---|---|---|---|
| $L$ | -593.54 | -592.23 | **-591.91** | -592.60 | -593.11 |
| $\chi^2$ | 6.127 | 3.632 | **3.077** | 4.324 | 5.265 |
| df | 2 | 2 | 2 | 2 | 2 |
| $p$-value | 0.04673 | 0.1627 | **0.2147** | 0.1151 | 0.07190 |
| RMSE | 5.154 | 2.969 | **2.923** | 3.565 | 4.398 |

18. The frequency of direct job changes from the German Socio-Economic Panel.

    Wagner, G.G., R.V. Burkhauser, and F. Behringer (1993). The English language public use file of the German Socio-Economic Panel. *Journal of Human Resources* 28, 429–433.

| value | 0 | 1 | 2 | 3 | 4 | 5 | 6 | 7 | 8 | 9 | 10 | 11 | 12 |
|---|---|---|---|---|---|---|---|---|---|---|---|---|---|
| frequency | 1333 | 404 | 133 | 43 | 25 | 10 | 4 | 4 | 1 | 2 | 2 | 0 | 1 |

$\overline{x} = 0.5398,\ s^2 = 1.179,\ b_1 = 3.729$
$D = 2.184, p_0^{\text{emp}} = 0.6794$

| | PIG | NLD | EDLID | ABM | LMNS |
|---|---|---|---|---|---|
| $L$ | -1934.33 | -1941.90 | -1949.14 | -1935.62 | **-1934.18** |
| $\chi^2$ | 1.691 | 11.06 | 21.66 | 3.407 | **1.608** |
| df | 4 | 4 | 4 | 4 | 4 |
| $p$-value | 0.7924 | 0.02586 | $< 0.001$ | 0.4921 | **0.8074** |
| RMSE | 2.997 | 10.47 | 14.04 | 5.874 | **2.740** |

19. Automobile claim data in Turkey, 2012-2014.

    Sarul, L.S. and S. Sahin (2015). An application of claim frequency data using zero inflated and Hurdle models in general insurance. *Journal of Business, Economics and Finance* 4(4), 732-743.

| value | 0 | 1 | 2 | 3 | 4 | 5 |
|---|---|---|---|---|---|---|
| frequency | 8544 | 1796 | 370 | 81 | 22 | 1 |

$\overline{x} = 0.2656,\ s^2 = 0.3347,\ b_1 = 2.574$
$D = 1.260, p_0^{\text{emp}} = 0.7901$

| | PIG | NLD | EDLID | ABM | LMNS |
|---|---|---|---|---|---|
| $L$ | -7033.13 | **-7031.28** | -7031.48 | -7031.57 | -7032.25 |
| $\chi^2$ | 1.312 | 0.3686 | 2.012 | **0.1400** | 0.4172 |
| df | 2 | 2 | 2 | 2 | 2 |
| $p$-value | 0.5188 | 0.8317 | 0.3657 | **0.9324** | 0.8117 |
| RMSE | 12.79 | 3.728 | 8.724 | **3.5159** | 7.513 |

20. The Central Sydney tai chi Trial (falls count data).

Ullah, S., C.F. Finch, and L. Day (2010). Statistical modelling for fall count data. *Accident Analysis and Prevention* 42, 384–392.

| value | 0 | 1 | 2 | 3 | 4 | 5 |
|---|---|---|---|---|---|---|
| frequency | 256 | 54 | 14 | 10 | 1 | 2 |

$$\overline{x} = 0.3739,\ s^2 = 0.6515,\ b_1 = 2.748$$
$$D = 1.742, p_0^{\text{emp}} = 0.7596$$

| | PIG | NLD | EDLID | ABM | LMNS |
|---|---|---|---|---|---|
| $L$ | -268.55 | **-267.87** | -267.93 | -268.06 | -268.36 |
| $\chi^2$ | 1.281 | 1.372 | 1.887 | **1.196** | 1.274 |
| df | 1 | 1 | 1 | 1 | 1 |
| $p$-value | 0.2577 | 0.2414 | 0.1695 | **0.2741** | 0.2591 |
| RMSE | 2.366 | 2.229 | 2.617 | **2.092** | 2.213 |
